# Supplementary material for: On the Privacy Risks of Model Explanations
Source: arXiv:1907.00164 source file (2021-02-05)
Supplement: Supplementary file 1 [file Appendix_Epochs.tex]

\section{Influence of overfitting}\label{app:overfitting}
To study the influence of overfitting on the success of membership inference attacks based on backpropagation-based methods, we trained models for varying epochs, which leads to varying gaps between training and testing accuracy. We used the same settings as for the experiments in Section~
\ref{sec:thresholdExperiments} as described in Appendix~\ref{app:datasets}. With the exception of the number of epochs we trained each target model, which we varied from 5 to 50 in steps 5. For each number of epochs we trained 20 target models. We only report the results for the optimal attack, as shadow model based attacks are similar. We only conducted experiments for \purchase, \texas, and \cifarTen where we had positive results for the highest amount of overfitting, which is achieved in the original setting. 

\begin{figure}
	\centering
	\if\compileFigures1
	\pgfplotstableread{data/feature/epochs.dat}{\epoch}
	\def\scale{0.5}
	\begin{tikzpicture}
	\begin{axis}[scale=\scale,yticklabel=
	{\pgfmathprintnumber\tick\%},
	axis y line*=left,
	ylabel={Attack accuracy},
	axis x line*=bottom,xlabel={Number of epochs},xmin=0,ymin=50,clip=false]	
	\addplot[color=blue,opacity=0.5,ultra thick] table [x={epochs}, y=purchase] {\epoch};
	\addplot[color=blue,opacity=0.75,ultra thick] table [x={epochs}, y=cifar10] {\epoch};
	\addplot[color=blue,opacity=1,ultra thick] table [x={epochs}, y=texas] {\epoch};
	\node at (axis cs:50,52) [anchor=west] {\color{blue}\cifarTen};
	\node at (axis cs:50,59) [anchor=west] {\color{blue}\purchase};
	\node at (axis cs:50,67) [anchor=west] {\color{blue}\texas};
	\end{axis}  
	\end{tikzpicture}
	\else
	\includegraphics[]{fig/\filename-figure\thefiguerNumber.pdf}
	\stepcounter{figuerNumber}
	\fi
	\caption{The attack accuracy of the attacker increases with increasing number of epochs.}
\end{figure}
