# Supplementary material for: On the Privacy Risks of Model Explanations
Source: arXiv:1907.00164 source file (2021-02-05)
Supplement: Supplementary file 2 [file Appendix_Lime.tex]

\subsection{Attacks using Lime explanation}\label{app:lime}
We ran additional experiments where the attacker has access to the Lime \cite{ribeiro2016programs} explanations. The type of attack is the same as described in Section~\ref{sec:thresholdDescription} (i.e. we use an optimal threshold based on the variance of the explanation). However, the calculation of Lime explanations takes considerably longer than the other explanations we considered. Each single explanation computes for a couple of seconds. Running experiments with 10,000 or more explanations would take weeks to months. To save time and energy we decided to run only some smaller scale experiments where the models are trained on 1,000 points and the attacks run on 2,000 points each (1,000 members and 1,000 non-members), we also repeated each experiment only 20 times instead of 100 as for the others. As the experiments for the other explanations indicated that only for \purchase and \texas the attack was likely to be successful we restricted our experiments to these two datasets. Figure~\ref{fig:lime} shows the results for these attacks, we also rerun the attacks for the gradient  and SmoothGrad explanations, as well as the attack using the prediction variance in this new setting, to ensure that it's not the different setting  that determines the outcome. Neither, Lime nor SmoothGrad outperform random guessing. For the \purchase dataset, however, the attack using the gradient variance fails as well. As a final interesting observation, we are unable to explain at the moment, for the \texas dataset the gradient based attack actually performs better than on the larger dataset (shown in Figure~\ref{fig:thresholdattacks}) it even outperforms the attack based on the prediction in this specific setting. Something we want to explore further in future works.

\begin{figure}
	\centering
	\if\compileFigures1
	\begin{tikzpicture}
	\begin{axis}[yscale=0.5,xscale=1,
	ymin=0,
	ybar=0.5pt,
	yticklabel=
	{\pgfmathprintnumber\tick\%},
	axis y line*=left,
	axis x line*=bottom,
	enlarge x limits=0.5,
	%legend style={at={(0.04,-0.4)},
	legend style={draw=none,at={(0.5,-0.4)},
		anchor= north,legend columns=1},
	ylabel={Attack accuracy},
	y label style={at={(axis description cs:0.06,1)},anchor=south},
	symbolic x coords={\texas,\purchase},
	xtick = {\texas,\purchase},
	legend columns=2, 
	clip=false,
	%xtick=data,
	%nodes near coords,
	%nodes near coords align={vertical},
	]
	
	\addplot[blue, fill ] coordinates {(\texas,84) (\purchase,51)};
	
	\addplot[bblue, fill ] coordinates {(\texas,69) (\purchase,67)};
	
	\addplot[red, fill, opacity=0.5] coordinates {(\texas,51) (\purchase,51) };
	
	\addplot[green, fill ] coordinates {(\texas,50) (\purchase,51) };

	\draw[thick, dashed] (-50,500) -- (150,500) node [black,sloped,above right,yshift=-2,xshift=-40]  {Random guess};
	\draw (630,520-50) node {Network};
	\legend{Gradient, Prediction, Lime, SmoothGrad}
	\end{axis}
	\end{tikzpicture}
	\else
	\includegraphics[]{fig/\filename-figure\thefiguerNumber.pdf}
	\stepcounter{figuerNumber}
	\fi
	\caption{Attacks using Lime or SmoothGrad do not outperform random guessing in any of our experiments.}
	\label{fig:lime}
\end{figure}
